# Supplementary material for: Keldysh effective action theory for universal physics in spin-1/2 Kondo dots
Source: arXiv:1203.4360 source file (2013-03-12)
Supplement: Supplementary file 1 [file paper_supp.pdf]

# Supplementary material for "Keldysh effective action theory for universal physics in spin-$\frac{1}{2}$ Kondo dots"

Sergey Smirnov* and Milena Grifoni
*Institut für Theoretische Physik, Universität Regensburg, D-93040 Regensburg, Germany*
(Dated: March 12, 2013)

## LOW TEMPERATURES AND VOLTAGES

At low energies, $T \ll T_{\mathrm{K}}$, $eV \ll kT_{\mathrm{K}}$, the differential conductance (see Ref. [14] of the main text),

$$G(T,V) = \pi\frac{e^2}{h}\frac{\partial}{\partial(eV)}\int_{-\infty}^{\infty} d\epsilon[n_{\mathrm{R}}(\epsilon) - n_{\mathrm{L}}(\epsilon)]\Gamma\nu_\sigma(\epsilon), \quad (1)$$

can be expanded around $T = 0$, $V = 0$. In Eq. (1)

$$n_{\mathrm{L,R}}(\epsilon) = \frac{1}{\exp(\frac{\epsilon-\mu_0 \pm eV/2}{kT}) + 1}. \quad (2)$$

Below we use $\mu_0 = 0$.

Let us define the following functions,

$$\begin{aligned} b_1(\epsilon,T,V) &\equiv \ln\left[\frac{1}{4\pi(T/T_{\mathrm{K}})}\right] - \\ &- \frac{1}{2}\sum_{s=\pm 1}\mathrm{Re}\,\psi\left[\frac{1}{2} + \frac{\mathcal{E}_\alpha}{2\pi(T/T_{\mathrm{K}})} + i\frac{seV/2+\epsilon}{2\pi kT}\right], \\ b_2(\epsilon,T,V) &\equiv \frac{\pi}{2} - \\ &- \frac{1}{2}\sum_{s=\pm 1}\mathrm{Im}\,\psi\left[\frac{1}{2} + \frac{\mathcal{E}_\alpha}{2\pi(T/T_{\mathrm{K}})} + i\frac{seV/2+\epsilon}{2\pi kT}\right], \\ g(\epsilon,T,V) &\equiv \frac{1}{[b_1(\epsilon,T,V)]^2 + [b_2(\epsilon,T,V)]^2}. \end{aligned} \quad (3)$$

At low energies one can write (see Eqs. (5) and (6) in the main text)

$$\Gamma\nu_\sigma(\epsilon) = \frac{\pi}{2}g(\epsilon,T,V). \quad (4)$$

At $V = 0$ we use the Sommerfeld expansion (N.W. Ashkroft and N.D. Mermin, *Solid State Physics* (Saunders College, Philadelphia, 1976)) and obtain

$$\begin{aligned} G(T,0) = \frac{\pi^2 e^2}{2h}\Big[&g(0,0,0) + g_T(0,0,0)T + \\ &+ \frac{1}{2}g_{TT}(0,0,0)T^2 + \frac{\pi^2}{6}(kT)^2 g_{\epsilon\epsilon}(0,0,0)\Big] + \mathcal{O}(T^4), \end{aligned} \quad (5)$$

where the lower index denotes the partial derivative with respect to the corresponding variable.

After straightforward calculations one finds

$$\begin{aligned} &g(0,0,0) = \frac{4}{\pi^2}, \quad g_T(0,0,0) = 0, \\ &g_{TT}(0,0,0) = -\frac{32}{3\pi^2}\frac{\ln(2|\mathcal{E}_\alpha|)}{|\mathcal{E}_\alpha|^2}\frac{1}{T_{\mathrm{K}}^2}, \\ &g_{\epsilon\epsilon}(0,0,0) = -\frac{32}{\pi^4}\frac{\ln(2|\mathcal{E}_\alpha|)+1}{|\mathcal{E}_\alpha|^2}\frac{1}{(kT_{\mathrm{K}})^2}. \end{aligned} \quad (6)$$

At $T = 0$ one can write

$$\begin{aligned} G(0,V) = \frac{\pi^2 e^2}{2h}\Big[&\frac{d}{d(eV)}\int_{-eV/2}^{eV/2} d\epsilon g(\epsilon,T,V)\Big|_{T=0,V=0} + \\ &+ \frac{(eV)^2}{2}\frac{d^3}{d(eV)^3}\int_{-eV/2}^{eV/2} d\epsilon g(\epsilon,T,V)\Big|_{T=0,V=0}\Big] + \\ &+ \mathcal{O}[(eV)^4]. \end{aligned} \quad (7)$$

Straightforward calculations lead to

$$\begin{aligned} &\frac{d}{d(eV)}\int_{-eV/2}^{eV/2} d\epsilon g(\epsilon,T,V)\Big|_{T=0,V=0} = \frac{4}{\pi^2}, \\ &\frac{d^3}{d(eV)^3}\int_{-eV/2}^{eV/2} d\epsilon g(\epsilon,T,V)\Big|_{T=0,V=0} = \\ &= \frac{1}{4}g_{\epsilon\epsilon}(0,0,0) + 3g_{(eV)(eV)}(0,0,0), \\ &g_{(eV)(eV)}(0,0,0) = -\frac{8}{\pi^4}\frac{\ln(2|\mathcal{E}_\alpha|)}{|\mathcal{E}_\alpha|^2}\frac{1}{(kT_{\mathrm{K}})^2}. \end{aligned} \quad (8)$$

From equations (5)-(8) one gets

$$\begin{aligned} G(T,V) = \frac{2e^2}{h}\Big[&1 - c_T\Big(\frac{T}{T_{\mathrm{K}}}\Big)^2 - c_V\Big(\frac{eV}{kT_{\mathrm{K}}}\Big)^2\Big] + \\ &+ \mathcal{O}[T^4, T^2(eV)^2, (eV)^4], \end{aligned} \quad (9)$$

where the Fermi liquid coefficients and their ratio are

$$c_T = \frac{4}{3}\frac{2\ln(2|\mathcal{E}_\alpha|)+1}{|\mathcal{E}_\alpha|^2}, \quad c_V = \frac{1}{\pi^2}\frac{4\ln(2|\mathcal{E}_\alpha|)+1}{|\mathcal{E}_\alpha|^2}, \quad (10)$$

$$\frac{c_V}{c_T} = \frac{3}{2\pi^2}\frac{4\ln(2|\mathcal{E}_\alpha|)+1}{4\ln(2|\mathcal{E}_\alpha|)+2}. \quad (11)$$

## LINEAR CONDUCTANCE AT HIGH TEMPERATURES

At temperatures above the Kondo temperature the universal behavior of the linear conductance (or the differential conductance maximum) $G(T)$ is well described by the expression obtained by Hamann [22],

$$G(T) = \frac{e^2}{h}\left(1 - \frac{\ln(T/T_{\mathrm{KH}})}{[\ln^2(T/T_{\mathrm{KH}}) + 3\pi^2/4]^{1/2}}\right), \quad (12)$$

where $T_{\mathrm{KH}} = \widetilde{T}_{\mathrm{K}}/1.2$.

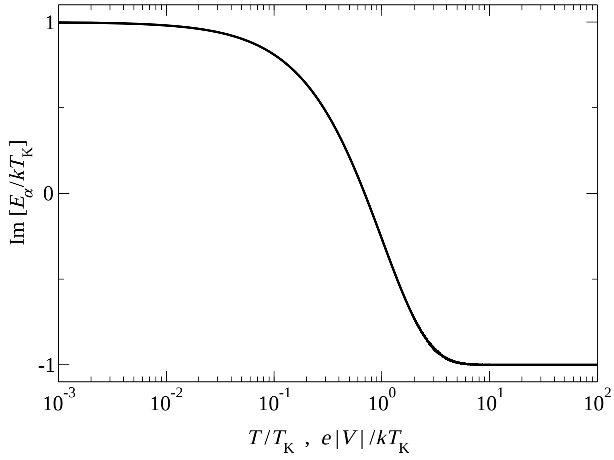


FIG. 1: A simple function of the temperature and bias voltage used for the imaginary part of the universal function $E_\alpha$.

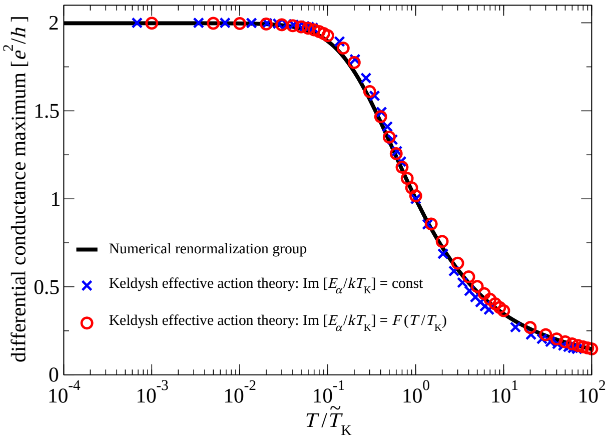


FIG. 2: The universal linear conductance as a function of the temperature. The NRG results (solid line) are provided by T. Costi and L. Merker (research center of Jülich).

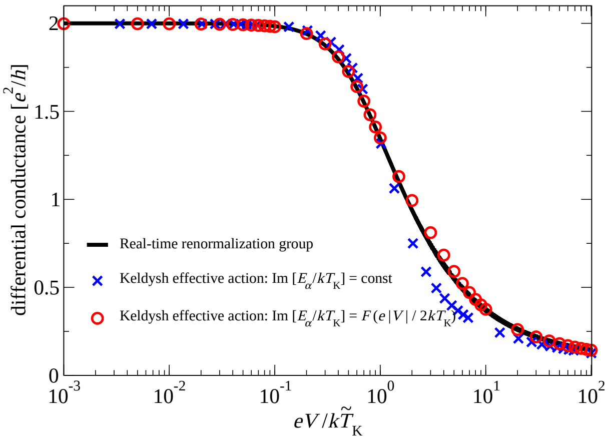


FIG. 3: The universal differential conductance as a function of the bias voltage at $T = 0$. The RTRG data are provided by M. Pletyukhov and H. Schoeller (University of Aachen).

This result was obtained for the s-d model where charge fluctuations are absent. In the Anderson model charge fluctuations are present. Using NRG, it was demonstrated in Ref. [26] that due to this difference Eq. (12) underestimates the conductance at very high temperatures. The high temperature asymptotic behavior of our theory agrees with Eq. (12). However, since our theory is based on the Anderson model, at very high temperatures, as expected, the linear conductance is larger than the one obtained from Eq. (12). This is in complete accordance with the NRG results of Ref. [26]. In our model the deviation from the Hamann's result develops at temperatures much higher than those in Ref. [26] because in those NRG calculations $U$ was finite, $U \approx 6\Gamma$, and the Anderson model was symmetric, $\mu_0 - \epsilon_d \approx 3\Gamma$. In our case $U = \infty$ and thus the Anderson model is highly asymmetric. We use $\mu_0 - \epsilon_d = 8\Gamma$. The asymmetry and charge fluctuations in this model become important at much higher temperatures.

## PHENOMENOLOGICAL EXPRESSION FOR THE UNIVERSAL FUNCTION

Here we show how the results presented in the main text may change if one assumes a temperature and voltage dependence of the universal function $\mathcal{E}_\alpha$. Namely, we keep the real part of $\mathcal{E}_\alpha$ constant with the same value as in the main text, $\mathcal{E}_\alpha^R \approx 1.42$, while the imaginary part is taken to be a simple monotonous function, $\mathcal{E}_\alpha^I = F(T/T_K)$ at $V = 0$ and $\mathcal{E}_\alpha^I = F(e|V|/kT_K)$ at $T = 0$. Here

$$F(x) = \frac{n_B(xkT) - 1}{n_B(xkT) + 1}, \tag{13}$$

where $n_B(\epsilon)$ is the Bose occupation number, $n_B(\epsilon) = [\exp(\epsilon/kT) - 1]^{-1}$. Using the Bose distribution one can rewrite the function $F(x)$ in a simple form,

$$F(x) = 2\exp(-x) - 1. \tag{14}$$

The imaginary part of $\mathcal{E}_\alpha$ as a function of $T/T_K$ (at $V = 0$) or $e|V|/kT_K$ (at $T = 0$) is shown in Fig. 1.

As one can see from Figs. 2 and 3, a temperature and voltage dependence, if any, of the imaginary part of the universal function $\mathcal{E}_\alpha$ may notably change the results presented in the main text for the highly asymmetric SIAM.

It is interesting to note that if the imaginary part of the universal function $\mathcal{E}_\alpha$ had the same dependence on the temperature and bias voltage, its impact on the equilibrium and nonequilibrium results would be similar.

* Electronic address: `sergey.smirnov@physik.uni-regensburg.de`
